# Supplementary material for: Understanding failures in electronic structure methods arising from the geometric phase effect
Source: arXiv:2411.08209 source file (2025-08-14)
Supplement: Supplementary file 1 [file SI_Understanding.pdf]

# Supporting Information for "Understanding failures in electronic structure methods arising from the geometric phase effect"

Eirik F. Kjønstad* and Henrik Koch*

*Department of Chemistry, Norwegian University of Science and Technology, NTNU, 7491 Trondheim, Norway*

E-mail: eirik.kjonstad@ntnu.no; henrik.koch@ntnu.no

# Ethylene

The MECI geometry is that reported in Ref. 1. In the scan, $h$ is orthogonalized against $g$ and normalized. The plot is produced by a 29x29 grid with matplotlib. To ensure a consistent solution, the scan was performed in a specific order, tracing out squares in clockwise and counter-clockwise directions starting at the outer edge and moving progressively towards the origin in $gh$ space. To obtain the positive and negative excitation energy solutions, the starting-position was chosen as largest-$g$/largest-$h$ (positive energy solution) and largest-$g$/smallest-$h$ (negative energy solution). If a scan along a square in either direction cannot converge (corresponding to a breakdown of the solution), the scan moves on to the next smaller square. To avoid jumps from one solution to another, the amplitudes at a given grid point was restarted with the amplitudes at the previous grid point, with orbital diabatization enabled in order to ensure correctly phased orbitals and thus consistent cluster amplitudes throughout the grid. The largest amplitude $t_{ai}$ is given by $i = 8$ and $a = 1$, where indices refer to the canonical energy-ordered Hartree-Fock orbitals in the initial geometries.

```
eps-meci.xyz
6

 H     1.058010228983    -0.482031642499     0.748682126808
 C     0.616740151636     0.131901054606    -0.063931545812
 H     1.352586208894     0.443326418094    -0.825198848590
 C    -0.773651435803     0.359987825494    -0.248758876785
 H    -1.385170907401     0.452809223074     0.677021634433
 H    -0.868614246311    -0.805992878768    -0.288214490056

g.xyz
6
```

```
  H      0.007313466289      0.057147259497      0.037233885635
  C      0.018065045039      0.010653044239      0.029770694182
  H     -0.011045778402     -0.044246241553     -0.025640855466
  C     -0.016011637809     -0.042775821534      0.029986440784
  H      0.030212324793     -0.002500610868      0.030496622594
  H     -0.028533419910      0.021722370219     -0.101846787729
```

```
h.xyz
6

  H      0.009983729150      0.004279864574      0.006085526830
  C     -0.059128405254     -0.031406366244      0.011698042309
  H     -0.000072261588     -0.004346978757     -0.005302673058
  C      0.013554961398      0.069990614294     -0.037047741578
  H      0.008830292504     -0.027241876753      0.014224759752
  H      0.027122442072     -0.011417198126      0.010473940680
```

# $HeH_2$

The scan was performed using orthonormalized $g$ and $h$ vectors ($h$ against $g$) and trace out a path about the intersection in polar coordinates with $r = 0.05$ and $\vartheta \in [0, 2\pi]$.

```
r0.xyz
3

 He       -3.0550286035       2.1141352239      -0.0000000000
 H        -3.0683904190       2.8140076850      -0.0000000000
```

```
 H       -1.4161794648       1.7355886604       0.0000000000
```

```
g.xyz
3

 He    -0.029179930000     0.252581195374    -0.000000000000
 H      0.039745642053    -0.269795429643     0.000000000000
 H     -0.010565712053     0.017214234269     0.000000000000
```

```
h.xyz
3

 He    -0.046895936222     0.018574090919    -0.000000000000
 H      0.038564774959    -0.033157681260     0.000000000000
 H      0.008327413423     0.014576364154     0.000000000000
```

## References


(1) Angelico, S.; Kjønstad, E. F.; Koch, H. Determining Minimum Energy Conical Intersections by Enveloping the Seam: Exploring Ground and Excited State Intersections in Coupled Cluster Theory. *J. Phys. Chem. Lett.* **2025**, *16*, 561–567.
